# Supplementary material for: Grain-boundary topological superconductor
Source: arXiv:2212.14038 ancillary file (2023-08-29)
Supplement: Supplementary file 1 [file SupplementaryInformation.pdf]

# Supplementary Information: "Grain-boundary topological superconductor"

Morten Amundsen
*Nordita, KTH Royal Institute of Technology and Stockholm University, Hannes Alfvéns väg 12, SE-106 91 Stockholm, Sweden*

Vladimir Juričić
*Nordita, KTH Royal Institute of Technology and Stockholm University, Hannes Alfvéns väg 12, SE-106 91 Stockholm, Sweden and Departamento de Física, Universidad Técnica Federico Santa María, Casilla 110, Valparaíso, Chile*

## Supplementary Note 1: Details of the numerical analysis

The model system consists of two square lattices, denoted left (L) and right (R), which are rotated in opposite directions by an angle $\alpha$, as seen in Supplementary Figure 1. The two lattices meet at the center line, marked in red, where the lattice mismatch causes an array of edge dislocations to form.

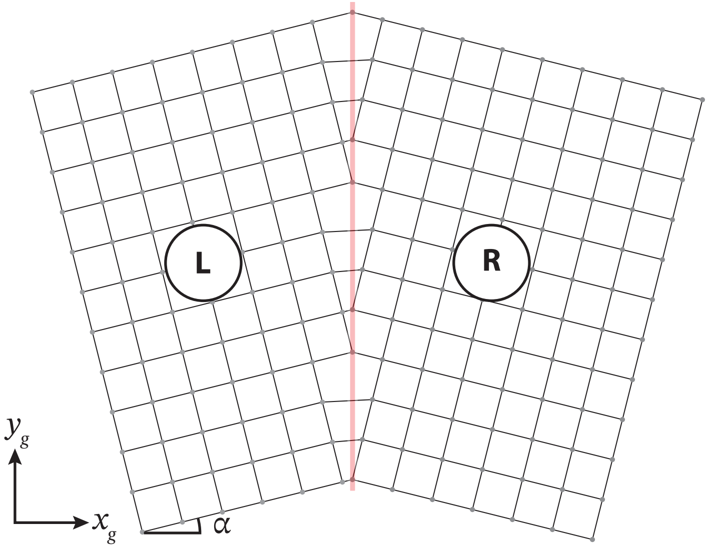


Supplementary Figure 1: Scaled down version of the lattice used in the numerical analysis. The red line indicates the location of the grain boundary. The labels L and R indicate the left and right sublattices, respectively, and $\alpha$ is the misalignment angle.

To establish a discretized real-space version of the Hamiltonian in Eq. (1) of the main text, we define the following Hamiltonian,

$$H = \frac{1}{2}\sum_{jl}\psi_j^\dagger \hat{H}_{jl}\psi_l, \tag{S1}$$

with Nambu vector at the lattice site $j$, $\psi_j = \begin{pmatrix} c_{j\uparrow} & c_{j\downarrow} & c_{j\uparrow}^\dagger & c_{j\downarrow}^\dagger \end{pmatrix}^\top$, and $\hat{H} = \hat{H}_0 + \hat{H}_p$, where $\hat{H}_0$ constitutes the non-superconducting part of the Hamiltonian,

$$\hat{H}_0 = \left[-t\left(\delta_{\hat{x}} + \delta_{-\hat{x}} + \delta_{\hat{y}} + \delta_{-\hat{y}}\right) + \left(4t-\mu\right)\delta_{jl}\right]\tau_3\sigma_0 - h_x\sigma_1\tau_3 - h_y\sigma_2\tau_0. \tag{S2}$$

In the above, $t = \hbar^2/2ma^2$, and we use the shorthand notation $\delta_{\hat{n}} \equiv \delta_{j+\hat{n},l}$. This contribution is independent of the lattice orientation. The superconducting part is assumed to be proximity-induced, and thus follows the global

coordinate system $(x_g, y_g)$. In the local coordinate systems of the two sublattices, one thus gets

$$\hat{H}_p^{L/R} = \frac{\Delta_p}{2ik_F a}\left[\left(\delta_{\hat{y}} - \delta_{-\hat{y}}\right)(\sigma_3\tau_1\cos\alpha \mp \sigma_0\tau_2\sin\alpha) - (\delta_{\hat{x}} - \delta_{-\hat{x}})(\sigma_0\tau_2\cos\alpha \pm \sigma_3\tau_1\sin\alpha)\right]. \quad \text{(S3)}$$

We note in particular that the grain boundary orientation aligns with the global $y_g$ axis.

The low-energy subspace of this Hamiltonian consists of both edge states and the states localized at the grain boundary. To isolate the latter, we discard eigenstates decaying in the direction parallel to the grain boundary. The remaining states are strongly peaked in the GB superlattice momentum space, as revealed by a discrete Fourier transform. By identifying this peak in the momentum for a given energy eigenvalue, the band structure can be established. The relevant band structures are shown in the upper panels in Fig. 1 of the main text, while additional plots are shown in Supplementary Figure 2.

## Supplementary Note 2: Additional plots

We here provide additional plots to support the discussion in the main text, see Supplementary Figure 2 and Supplementary Figure 3.

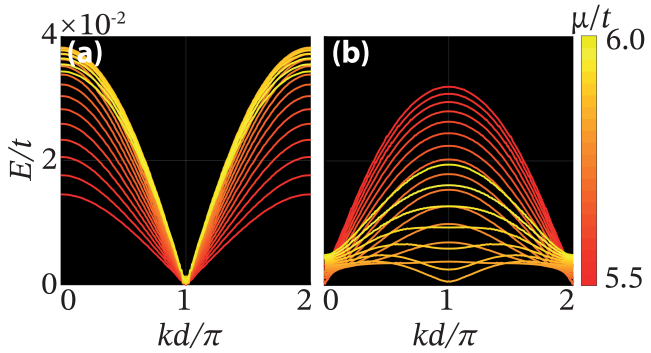


Supplementary Figure 2: Effect of the chemical potential $\mu$ (given in units of the hopping parameter $t$) on the grain boundary band structure for $d = 12a$ (the distance between edge dislocations on the same sublattice), where $a$ is the lattice spacing of the parent lattice, and (a) no slip between the sublattices (slip length $l = d/2$), (b) a slip of $l = 5d/12$. In the former case, there is always a node at $kd/\pi = 1$. In the latter case, the grain boundary band structure oscillates between featuring a node at either $kd/\pi = 0$ or 1, being gapped in between, and even featuring a flat band.

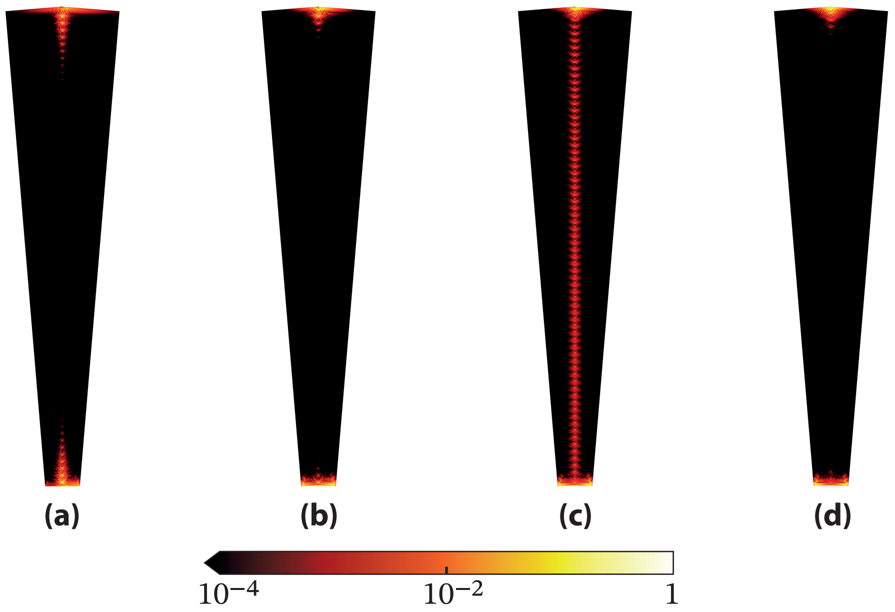


Supplementary Figure 3: Local density of states of the full geometry, corresponding to the truncated versions presented in Fig. 2 of the main text. The color code is the same as in Fig. 2 of the main text.

## Supplementary Note 3: Analytical form of the single-dislocation modes

We derive the form of the single-dislocation Majorana zero modes (MZMs) for the parent SC [Eq. (1) in the main text], which we here rewrite in the absence of the exchange field ($\boldsymbol{h} = 0$) for completeness. This Hamiltonian, in the basis $(c_{k,\uparrow}, c_{k,\downarrow}, c^\dagger_{-k,\uparrow}, c^\dagger_{-k,\downarrow})^\top$, where $c_{k,\uparrow}$, where $(c^\dagger_{k,\downarrow})$ is the annihilation (creation) operator for the quasiparticle with spin up (down) and momentum $\mathbf{k}$, reads as

$$H = \left[2t(2-\cos k_x a - \cos k_y a) - \mu\right]\sigma_0\tau_3 + \Delta_p\left(-\sin k_x a\,\sigma_0\tau_2 + \sin k_y a\,\sigma_3\tau_1\right), \tag{S4}$$

where $(\sigma_0, \boldsymbol{\sigma})$ $[(\tau_0, \boldsymbol{\tau})]$, are the standard Pauli matrices acting in the spin (Nambu) space, $t$ is the overall energy scale, $\mu > 0$ is the effective chemical potential, and $\Delta_p$ is the the $p-$wave pairing amplitude [1]. The obtained dislocation MZMs will be subsequently used as the Wannier basis for the SC state on the GB defect, in Supplementary Note 4. The analytical form of the modes can be found in the vicinity of the gap closing at the $M$ point in the Brillouin zone, but its overall form does not change throughout the translationally-active topological phase due to the continuity.

We consider a single-dislocation defect with the Burgers vector $\mathbf{b} = a\mathbf{e}_x$, which is introduced in the Volterra construction by removing the semi-infinite line of atoms at $x = 0$ which ends at the center of the defect located at the origin, for concreteness. This defect sources a $\pi$ flux, since the Fermi surface of the topological SC encloses the $M$ point at $\mathbf{K}_M = (\pi,\pi)/a$, and therefore $\Phi = \mathbf{K}_M \cdot \mathbf{b} = \pi$. The defect connects two edges at $x = \pm a$ with respect to the removed line, and ends at the center of the defect. The Hamiltonian of the two connected edges, obtained from Eq. (S4) by expanding about the momentum $\mathbf{K}_M$, keeping only the $x$-dependent terms (parallel to $\mathbf{b}$) and going back to the real space, is of the form

$$H_{\text{edge}} = (t\partial_x^2 + \tilde{\mu})\sigma_0\tau_3\rho_3 - i\Delta_p\partial_x\sigma_0\tau_2\rho_3. \tag{S5}$$

Here, $\tilde{\mu} = 8t - \mu$ being positive (negative) in the topological (trivial) phase, with $t > 0$, $\mu > 0$, the $\boldsymbol{\rho}$ Pauli matrices acting in the subspace of two edges at $x = \pm a$, each of which featuring a Kramers pair of the MZMs due to time-reversal symmetry. The dislocation MZM is the result of the topological frustration introduced by the dislocation defect, sourcing the flux $\Phi = \pi$ in a translationally-active topological phase, which is modelled by the term

$$H_{\text{D}} = \Delta_p\,\text{sign}x\,\sigma_0\tau_2\rho_2, \tag{S6}$$

so that the low-energy quasiparticles pick up a $\pi$ phase when crossing the dislocation defect, while it is $\sim \tau_2\rho_2$ to ensure the time-reversal symmetry and to preserve the form of the pairing along the Volterra cut (parallel to the Burgers vector). sign$(x)$ is the usual sign function. The spin part is $\sim \sigma_0$, and we can therefore omit for now.

We now solve for the zero modes of the Hamiltonian $H_{\text{edge}} + H_{\text{D}}$,

$$(H_{\text{edge}} + H_{\text{D}})\Psi_0(x) = 0, \tag{S7}$$

taking the ansatz consistent with the normalizability of the zero-mode state,

$$\Psi_0(x) \sim e^{-\lambda|x|}\chi_\alpha\varphi_\beta, \tag{S8}$$

where the two-component spinors $\chi$ and $\varphi$ act in the Nambu and the edge subspaces, respectively. The closed analytic form is then obtained following the steps analogous as in Ref. [2], and the solution reads as

$$\Psi_0(x) = \mathscr{C}\chi_{\text{sign}\,x}\,\varphi_{+1}\left(e^{-\lambda_1|x|} - e^{-\lambda_2|x|}\right), \tag{S9}$$

with $\mathscr{C}$ as the normalization constant, where the spinors $\chi$ and $\varphi$ satisfy

$$\tau_1\chi_\alpha = -\alpha\chi_\alpha, \quad \rho_1\varphi_\beta = \beta\varphi_\beta, \tag{S10}$$

and, for $\Delta_p \ll \tilde{\mu}$,

$$\lambda_{1,2} = \frac{\Delta_p}{2t} \pm i\sqrt{\frac{\tilde{\mu}}{t}} = \frac{\Delta_p k_F^2}{2\tilde{\mu}} \pm ik_F \equiv \kappa \pm ik_F. \tag{S11}$$

The last identity is obtained from Eq. (S5), by identifying $tk_F^2 = \tilde{\mu}$. Notice that $\rho_1 = \boldsymbol{\rho}\cdot\mathbf{b}/|\mathbf{b}|$, and thus the spinor in the edge subspace is locked to the Burgers vector. Therefore, we can write the zero-mode solution localized at the defect center, given by Eq. (S9), as

$$\Psi_0(x) = \mathscr{C}\chi_{\text{sign}\,x}\,\varphi_{+1}e^{-\kappa|x|}\sin k_F|x|. \tag{S12}$$

In the final step, we reintroduce the spin degree of freedom by recalling that the left edge with the spin up (down) corresponds to the right edge with the spin down (up). This allows us to effectively replace the edge subspace with the spin subspace, and therefore write the Kramers pair of the MZMs as

$$\Psi_{0,\pm}(x) = \sqrt{2\kappa}\,\Sigma_\pm\,\chi_{\text{sign}\,x}\,e^{-\kappa|x|}\sin k_F|x| \equiv \Sigma_\pm\,\chi_{\text{sign}\,x}\,f(x), \tag{S13}$$

where the spinor $\Sigma_\pm$

$$\frac{\boldsymbol{\sigma}\cdot\mathbf{b}}{|\mathbf{b}|}\Sigma_\pm = \pm\Sigma_\pm. \tag{S14}$$

Therefore, when the topological edge modes involve the spin explicitly, the dislocation zero-modes appear with the spin locked to the Burgers vector. Explicitly, for $x > 0$, the Kramers pair of the MZMs is of the form

$$\Psi_{0,+} = \frac{i}{2}f(x)\begin{pmatrix}1\\1\\-1\\-1\end{pmatrix},\quad \Psi_{0,-} = \frac{i}{2}f(x)\begin{pmatrix}1\\-1\\-1\\1\end{pmatrix}. \tag{S15}$$

To construct the Wannier basis of the MZMs, we will use the above pair of the zero modes, with same form along the grain boundary ($y$) direction, as orthogonal to it, which should be a good approximation at least at low energies, which is the regime we are after. The corresponding operators that annihilate the localized dislocation mode at the origin are directly obtained from Eq. S15, and read

$$\gamma_+ = \frac{i}{2}\int dy f(y)(c_{y,\uparrow}+c_{y,\downarrow}-c^\dagger_{y,\uparrow}-c^\dagger_{y,\downarrow}) = \gamma^\dagger_+,\quad \gamma_- = \frac{i}{2}\int dy f(y)(c_{y,\uparrow}-c_{y,\downarrow}-c^\dagger_{y,\uparrow}+c^\dagger_{y,\downarrow}) = \gamma^\dagger_-, \tag{S16}$$

confirming their Majorana form.

## Supplementary Note 4: Derivation of the effective model

To derive an effective tight-binding model along the GB defect, we take a basis of the Wannier states formed by the localized single-dislocation modes, given by Eq. (S16), which form the GB superlattice. From the form in Eq. (S16), we obtain the zero-energy states localized at an edge dislocation, with a Burgers vector pointing at an angle $\alpha$ with respect to the $x$ axis, in the form

$$|\psi_a(y)\rangle = \sqrt{2\kappa}\phi_a(\alpha)e^{-\kappa|y|}\sin k_F|y|, \tag{S17}$$

with $a = 1,2$, and

$$\phi_1(\alpha) = \frac{1}{2}\begin{pmatrix}e^{-i\alpha/2}\\e^{i\alpha/2}\\-e^{i\alpha/2}\\-e^{-i\alpha/2}\end{pmatrix},\quad \phi_2(\alpha) = \frac{1}{2}\begin{pmatrix}e^{-i\alpha/2}\\-e^{i\alpha/2}\\-e^{i\alpha/2}\\e^{-i\alpha/2}\end{pmatrix}.$$

To obtain the above form of the basis states, we use that the rotation by an angle $\alpha$ about the $z-$axis is represented on the particle-like [hole-like] components of the Nambu spinor by $R(\alpha)$ [$R^*(\alpha)$], where $R(\alpha) = e^{i\alpha\sigma_3/2}$. Notice that the opening angle of the GB defect is equal to $2\alpha$, and therefore the states at the left (right) side of the grain boundary are obtained rotating the dislocation states by an angle $\alpha$ ($\pi-\alpha$). One can now readily check that these modes are also Majoranas, analogously as in Eq. (S16).

We obtain the effective one-dimensional tight-binding Hamiltonian by projecting the parent Hamiltonian (Eq. (1) in the main text) on the basis formed by dislocation Wannier states at the left and right sublattices $a$ and $b$, respectively,

$$\begin{aligned}H_{gb} = \sum_j \Big[&\langle\psi_\alpha(y)|H|\psi_\alpha(y)\rangle\, a^\dagger_j a_j + \langle\psi_{\pi-\alpha}(y)|H|\psi_{\pi-\alpha}(y)\rangle\, b^\dagger_j b_j\\ &\langle\psi_\alpha(y+d)|H|\psi_\alpha(y)\rangle\, a^\dagger_{j+1}a_j + \langle\psi_{\pi-\alpha}(y+d)|H|\psi_{\pi-\alpha}(y)\rangle\, b^\dagger_{j+1}b_j\\ &\langle\psi_{\pi-\alpha}(y+ld)|H|\psi_\alpha(y)\rangle\, b^\dagger_j a_j + \langle\psi_\alpha(y+d)|H|\psi_{\pi-\alpha}(y+ld)\rangle\, a^\dagger_{j+1}b_j + \text{h.c.}\Big].\end{aligned} \tag{S18}$$

Hereafter the length of the slip, $l$, is expressed in units of the parameter $d$, the distance between edge dislocations on

the same sublattice. The corresponding matrices read as

$$\langle\psi_\alpha(y)|H|\psi_\alpha(y)\rangle = \begin{pmatrix} 0 & ih\sin(\alpha-\theta) \\ -ih\sin(\alpha-\theta) & 0 \end{pmatrix}, \tag{S19}$$

$$\langle\psi_{\pi-\alpha}(y)|H|\psi_{\pi-\alpha}(y)\rangle = \begin{pmatrix} 0 & ih\sin(\alpha+\theta) \\ -ih\sin(\alpha+\theta) & 0 \end{pmatrix}, \tag{S20}$$

$$\langle\psi_\alpha(y+d)|H|\psi_\alpha(y)\rangle \simeq \begin{pmatrix} 0 & +i\tilde{\Delta}(d) \\ +i\Delta\tilde{(d)} & 0 \end{pmatrix}, \tag{S21}$$

$$\langle\psi_{\pi-\alpha}(y+d)|H|\psi_{\pi-\alpha}(y)\rangle \simeq \begin{pmatrix} 0 & -i\tilde{\Delta}(d) \\ -i\tilde{\Delta}(d) & 0 \end{pmatrix}, \tag{S22}$$

$$\langle\psi_{\pi-\alpha}(y+ld)|H|\psi_\alpha(y)\rangle \simeq \begin{pmatrix} 0 & -i\tilde{\mu}(ld)+i\tilde{h}(ld)\cos\theta \\ -i\mu\tilde{(l}d)-i\tilde{h}(ld)\cos\theta & 0 \end{pmatrix} \tag{S23}$$

$$\psi_\alpha(y+d)|H|\psi_{\pi-\alpha}(y+ld) \simeq \begin{pmatrix} 0 & i\tilde{\mu}((1-l)d)+i\tilde{h}((1-l)d)\cos\theta \\ i\tilde{\mu}((1-l)d)-i\tilde{h}((1-l)d)\cos\theta & 0 \end{pmatrix}, \tag{S24}$$

with $\tilde{\Delta}(d) = \Gamma_1(d)\Delta\cos\alpha$, $\tilde{\mu}(ld) = (\Gamma_2(ld)+\Gamma_0(ld))\,\mu\cos\alpha$, and $\tilde{h}(ld) = \Gamma_0(ld)h$, where

$$\Gamma_n(z) = \frac{2\kappa}{k_F^n}\int_{-\infty}^{\infty} e^{-\kappa|y+z|}\sin k_F|y+z|\partial_y^n e^{-\kappa|y|}\sin k_F|y|\,dy, \tag{S25}$$

so that

$$\Gamma_0(z) \simeq e^{-\kappa z}\left[(1-\kappa z)\cos k_F z + \frac{2\kappa}{k_F}\sin k_F z\right], \tag{S26}$$

$$\Gamma_1(z) \simeq e^{-\kappa z}\left[(1-\kappa z)\sin k_F z - \frac{\kappa^2 z}{k_F}\cos k_F z\right] \tag{S27}$$

$$\Gamma_2(z) \simeq -e^{-\kappa z}\left[(1-\kappa z)\cos k_F z + \frac{2\kappa}{k_F}(1-\kappa d)\sin k_F z\right] \tag{S28}$$

$$\Gamma_2(z)+\Gamma_0(z) \simeq \frac{2\kappa^2 d}{k_F}e^{-\kappa z}\sin k_F z. \tag{S29}$$

Upon Fourier transforming, we thus obtain

$$H = \begin{pmatrix} 0 & 2\tilde{\Delta}(d)\sin kd + ih\sin(\alpha-\theta) & 0 & -i\,((W(k)-V(k)) \\ 2\tilde{\Delta}\sin kd - ih\sin(\alpha-\theta) & 0 & -i\,(W(k)+V(k)) & 0 \\ 0 & i\,(W^*(k)+V^*(k)) & 0 & -2\tilde{\Delta}\sin kd + ih\sin(\alpha+\theta) \\ i\,(W^*(k)-V^*(k)) & 0 & -2\tilde{\Delta}\sin kd - ih\sin(\alpha+\theta) & 0 \end{pmatrix}, \tag{S30}$$

where

$$W(k) = e^{ikld}\left[\tilde{\mu}(ld)+\tilde{\mu}((1-l)d)e^{-ikd}\right] = W^*(-k), \tag{S31}$$

$$V(k) = e^{ikld}\left[\tilde{h}(ld)+\tilde{h}((1-l)d)e^{-ikd}\right]\cos\theta = V^*(-k). \tag{S32}$$

The last two equation imply that the real and the imaginary parts of the functions $W(k)$ and $V(k)$ satisfy

$$\mathrm{Re}\,W(k) = \mathrm{Re}\,W(-k),\ \ \mathrm{Im}\,W(k) = -\mathrm{Im}\,W(-k), \tag{S33}$$

$$\mathrm{Re}\,V(k) = \mathrm{Re}\,V(-k),\ \ \mathrm{Im}\,V(k) = -\mathrm{Im}\,V(-k). \tag{S34}$$

Eq. (S30) is unitarily equivalent to the form manifestly particle-hole symmetric,

$$H = \begin{pmatrix} 2\tilde{\Delta}\sin kd & -iW(k) & ih\sin(\alpha-\theta) & iV(k) \\ iW^*(k) & -2\tilde{\Delta}\sin kd & iV^*(k) & ih\sin(\alpha+\theta) \\ -ih\sin(\alpha-\theta) & -iV(k) & 2\tilde{\Delta}\sin kd & -iW(k) \\ -iV^*(k) & -ih\sin(\alpha+\theta) & iW^*(k) & -2\tilde{\Delta}\sin kd \end{pmatrix} \equiv \begin{pmatrix} H_0(k) & P(k) \\ P^\dagger(k) & -H_0^\top(-k) \end{pmatrix}, \tag{S35}$$

where

$$H_0(k) = \begin{pmatrix} 2\tilde{\Delta}\sin kd & -iW(k) \\ iW^*(k) & -2\tilde{\Delta}\sin kd \end{pmatrix},\ \ P(k) = ih\begin{pmatrix} \sin(\alpha-\theta) & \tilde{V}(k) \\ \tilde{V}^*(k) & \sin(\alpha+\theta) \end{pmatrix}, \tag{S36}$$

which is the form of Eq. (2) in the main text.

## Supplementary Note 5: $\mathbb{Z}_2$ Topological Invariant & the magnetic-field induced topological phase transitions

Our system is in symmetry class $D$, for which the topological invariant is found from the product of the Pfaffians of Eq. (S35) evaluated at the $\Gamma$ and $M$ points. For a matrix of the block form

$$A_1 = \begin{pmatrix} B & C \\ -C^T & D \end{pmatrix}, \tag{S37}$$

the Pfaffian is given as

$$\mathrm{Pf}(A_1) = \mathrm{Pf}(B)\mathrm{Pf}\big(D + C^T B^{-1} C\big). \tag{S38}$$

Furthermore, for an antisymmetric $2\times 2$ matrix of the form

$$A_2 = \begin{pmatrix} 0 & \alpha a \\ -\alpha a & 0 \end{pmatrix}, \tag{S39}$$

its Pfaffian is given by

$$\mathrm{Pf}(A_2) = a. \tag{S40}$$

Hamiltonian in Eq. (S35) at the time-reversal symmetric $\Gamma$ and $M$ points in the superlattice BZ is antisymmetric, and therefore the Pfaffian is well defined, as it should be for a Majorana Hamiltonian. Using the above identities, we obtain the following expressions for the Pfaffians,

$$P(\Gamma) = \big(\tilde{\mu}(ld) + \tilde{\mu}((1-l)d)\big)^2 - \big(\tilde{h}(ld) + \tilde{h}((1-l)d)\big)^2 \cos\theta + h^2 \sin(\alpha+\theta)\sin(\alpha-\theta), \tag{S41}$$

$$P(M) = \big(\tilde{\mu}(ld) - \tilde{\mu}((1-l)d)\big)^2 - \big(\tilde{h}(ld) - \tilde{h}((1-l)d)\big)^2 \cos\theta + h^2 \sin(\alpha+\theta)\sin(\alpha-\theta). \tag{S42}$$

The topological invariant may now be found as [3]

$$(-1)^\nu = \mathrm{sgn}\,[P(\Gamma)P(M)]\,. \tag{S43}$$

For $\theta = 0$ (the exchange field orthogonal to the GB), these expressions reduce to

$$P(\Gamma) = \big(\tilde{\mu}(ld) + \tilde{\mu}((1-l)d)\big)^2 - \big(\tilde{h}(ld) + \tilde{h}((1-l)d)\big)^2 + h^2 \sin^2\alpha, \tag{S44}$$

$$P(M) = \big(\tilde{\mu}(ld) - \tilde{\mu}((1-l)d)\big)^2 - \big(\tilde{h}(ld) - \tilde{h}((1-l)d)\big)^2 + h^2 \sin^2\alpha, \tag{S45}$$

both of which can become negative, owing to the second term in each expression. However, this is excluded, as this term is exponentially suppressed, see Eq. (S26), and, moreover, the exchange field is rather weak. On the other hand, for $\theta = \pi/2$, we get

$$P(\Gamma) = \big(\tilde{\mu}(ld) + \tilde{\mu}((1-l)d)\big)^2 - h^2\cos^2\alpha, \tag{S46}$$

$$P(M) = \big(\tilde{\mu}(ld) - \tilde{\mu}((1-l)d)\big)^2 - h^2\cos^2\alpha. \tag{S47}$$

In the notation used in the main text, where $t_{ab} = \tilde{\mu}(ld)$, and $t_{ba} = \tilde{\mu}((1-l)d)$, we find the topological invariant in this case to be

$$(-1)^\nu = \mathrm{sgn}\left[\big((t_{ab}+t_{ba}) - h^2\cos^2\alpha\big)\big((t_{ab}-t_{ba}) - h^2\cos^2\alpha\big)\right]. \tag{S48}$$

Hence, a topologically nontrivial regime, $\nu = 1$, is realized for

$$t_{\min} < h\cos\alpha < t_{\max}, \tag{S49}$$

where $t_{\min}$ ($t_{\max}$) = min(max) $\{|t_{ab}-t_{ba}|, |t_{ab}+t_{ba}|\}$. At the same time, as can be readily seen from Eq. (S35), $t_{\min}$ ($t_{\max}$) is minimum (maximum) gap of the grain-boundary SC in the absence of the exchange field, $\boldsymbol{h} = 0$.

We now compute the critical angles for the topological transition based on the previous topological analysis of the effective model. We consider the parameter regime in Figs. 2-4 in the main text, where the gap closes at the $\Gamma$ point, and the topological phase transition takes place through the sign change of the Pfaffian at the $\Gamma$ point, as well. We first use Eq. (S46) for the exchange field along the grain boundary ($\theta = \pi/2$) to find that the critical exchange field in this case is

$$h_{\mathrm{crit}} = \frac{t_{ab}+t_{ba}}{\cos^2\alpha}. \tag{S50}$$

We then take Eq. (S41) to calculate the critical angles for the topological transition at the fixed magnitude of the exchange field, reported in Fig. 4(b) of the main text. Neglecting the contribution $\tilde{h}$ in Eq. (S41), as being exponentially suppressed by the superlattice constant [Eq. (S26)], Eq. (S41), together with Eq. (S50), yields the critical angle for the topological transition,

$$h_{\rm crit}^2 \cos^2\alpha + h^2 \sin(\alpha+\theta_c)\sin(\alpha-\theta_c) = 0, \tag{S51}$$

which has two solutions $\theta_{c,1} \simeq 57° = 1.00$ radians and $\theta_{c,2} \simeq 123° = 2.14$ radians, when the critical field is $h_{\rm crit} = 0.25t$, the applied field is $h = 0.3t$, and the grain boundary angle is $\alpha \simeq 4.8°$, as announced in the main text.

## Supplementary Note 6: Antiunitary symmetry of the effective grain-boundary Hamiltonian

The effective Hamiltonian in Eq. (S35) can be rewritten as

$$\begin{aligned} H(k) = {} & 2\tilde{\Delta}\sin kd\sigma_0\otimes\sigma_3 + {\rm Re\,W(k)}\sigma_0\otimes\sigma_2 + {\rm Im\,W(k)}\sigma_0\otimes\sigma_1 - h\sin(\alpha-\theta)\sigma_2\otimes\sigma_+ - h\sin(\alpha+\theta)\sigma_2\otimes\sigma_- \\ & - {\rm Re\,V(k)}\sigma_2\otimes\sigma_1 + {\rm Im\,W(k)}\sigma_2\otimes\sigma_2, \end{aligned} \tag{S52}$$

where $\sigma_\pm = (\sigma_0 \pm \sigma_3)/2$, which, together with Eqs. (S33) and (S34), implies that $H^*(k) = -H(-k)$, since momentum is odd under the (antiunitary) complex conjugation. Furthermore, the form of the Hamiltonian in Eq. S52 implies that $[H(k), \sigma_2\otimes\sigma_0] = 0$. Therefore, the effective GB Hamiltonian in Eq. S52 possesses an effective antiunitary particle-hole-like symmetry represented by the operator $U = (\sigma_2\otimes\sigma_0){\rm K}$, with $U^2 = -1$ and K as the complex conjugation, $UHU^\dagger = -H$, which explicitly reads

$$(\sigma_2\otimes\sigma_0)H^*(k)(\sigma_2\otimes\sigma_0) = -H(-k). \tag{S53}$$

Therefore, zero energy modes of this Hamiltonian form pairs, with each pair constituted by mutually orthogonal modes. In particular, this implies that the cohabitating topological MZMs are mutually orthogonal and therefore protected against hybridization even though they occupy the same end of the GB defect.

## Supplementary Note 7: Stability of the Majorana modes

In this section we demonstrate the stability of the zero-energy modes in the non-trivial phase. To do this, we introduce disorder via a random variation of the chemical potential, so that at a particular lattice point $i$, the chemical potential $\mu_i = \mu(1+\delta_i)$, where $\delta_i \in [-0.1, +0.1]$, thus giving a 10 % variation. The zero-energy local density of states is shown in Supplementary Figure 4 for two configurations. In (a) the chemical potential has the same variation throughout the entire lattice, whereas in (b), there is variation only in one of the sublattices - to make absolutely certain that there is no mirror symmetry. In both cases, four zero-energy modes remain, two of which are localized at the top of the grain boundary.

## Supplementary References


[1] Asahi, D. & Nagaosa, N. Topological indices, defects, and majorana fermions in chiral superconductors. *Phys. Rev. B* **86**, 100504 (2012).

[2] Roy, B. & Juričić, V. Dislocation as a bulk probe of higher-order topological insulators. *Phys. Rev. Res.* **3**, 033107 (2021).

[3] Kitaev, A. Y. Unpaired majorana fermions in quantum wires. *Phys.-Usp.* **44**, 131 (2001).

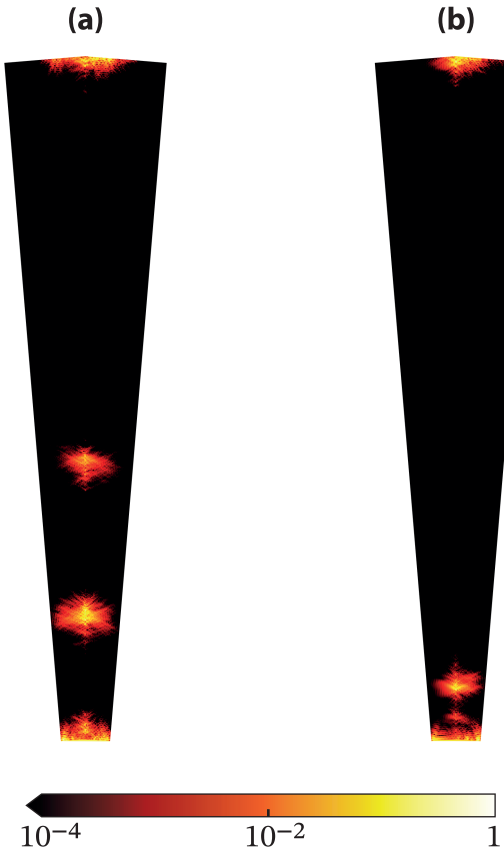


Supplementary Figure 4: Zero-energy local density of states in the presence of impurities, as modeled by a spatially varying chemical potential. In (a), the chemical potential varies throughout the system. In (b) the chemical potential varies only in one of the sublattices, and is constant in the other.
